# Supplementary material for: Depth Is All You Need for Monocular 3D Detection
Source: arXiv:2210.02493 source file (2022-10-05)
Supplement: Supplementary file 1 [file X_supplemental.tex]

\clearpage

\addtolength{\oddsidemargin}{-.7in}
\addtolength{\textwidth}{1.4in}
\addtolength{\columnsep}{0.2in}
\nolinenumbers

\appendix

% --- repeat the title 
\twocolumn[
\centering
\Large
\textbf{DD3Dv2: Depth is All You Need for 3D Detection} \\
\vspace{0.5em}Supplementary Material \\
\vspace{1.0em}
] %< twocolumn
\appendix

% --- PDF will be split by an editor (e.g. macOS preview), so need to restart from page 1
\setcounter{page}{1}

\section{KITTI ablation}
%In Table~\ref{tab:kitti_ablation}, we present a comparison between the two proposed approaches: multi-task using point-cloud vs. pseudo-labels from self-supervised depth, on the KITTI3D dataset. To this end, we use the standard \emph{train} and \emph{val} dataset splits, as introduced by \cite{chen2015monocular}. 
In Table~\ref{tab:kitti_ablation}, we evaluate our best method, multi-task using point-cloud, on the KITTI3D dataset. To this end, we use the standard \emph{train} and \emph{val} dataset splits, as introduced by \cite{chen2015monocular}. 

\begin{table}[h]
\centering
{
\begin{tabular}{l|c|c|c}
\thead{Adaptation \\ strategies} & \multicolumn{3}{c}{\thead{Detection Accuracy \\ BEV AP $\uparrow$ \darkgray{(Box AP [$\%$]$\uparrow$)}} }\\
& Car & Ped. & Cyc.\\
\midrule
% https://wandb.ai/tri/multitask/runs/2x2fl267
\small{\thead{DD3Dv2 \\ \small{(no-depth)}}} & 33.5 \darkgray{(24.4)}&13.2 \darkgray{(11.0)}&4.1 \darkgray{(3.7)} \\
\midrule
\multicolumn{4}{c}{\small{\textbf{Multi-task} (single stage)}} \\
\midrule
% https://wandb.ai/tri/multitask/runs/141h42xe
Supervised  & 
34.0 \darkgray{(25.0)}&
15.3 \darkgray{(12.9)}&
7.4 \darkgray{(6.3)} \\
%\midrule
%\multicolumn{4}{c}{\small{\textbf{Pseudo-labels $\rightarrow$ Multi-task}}} \\
%\midrule
%Self-supervised & xx.x \darkgray{(xx.x)}&xx.x \darkgray{(xx.x)}&xx.x \darkgray{(xx.x)} \\ 
% TODO: paste a wandb link
\end{tabular}

\vspace{1em}

\caption{\textbf{Ablation on KITTI.} We present an abridged version of Table~\ref{tab:ablation}, but now on KITTI 3D dataset.}
\label{tab:kitti_ablation}
}
\vspace{-5mm}
\end{table}

%The conclusion of this experiment is consistent with the analysis on the nuScenes dataset. When the depth representation is adapted using in-domain point-cloud data via multi-task training (i.e. DD3Dv2), we observe a clear improvement over the single-task baseline. When trained with pseudo-labels generated from a self-supervised depth predictor, we observe a competitive performance. 
When the depth representation is adapted using in-domain point-cloud data via multi-task training (i.e. DD3Dv2), we observe a clear improvement over the single-task baseline.

\section{Comparison with DD3D}
In Sec.~\ref{sec:dd3dv2}, we introduce a few modifications to the original DD3D~\cite{park2021dd3d} to facilitate multi-task training. To better quantify the effect of these modifications and to isolate the effect of our proposed adaptation methods, we evaluate DD3D using identical training parameters as described in Sec.~\ref{sec:ablation}\footnote{This experiment uses the publicly available implementation: \url{https://github.com/TRI-ML/dd3d}}; $60K$ SGD steps and $32$ as the batch size (Table~\ref{tab:orig_dd3d}). When trained using this \emph{short} training schedule, DD3Dv2 outperforms DD3D by 4.9\% in NDS. We argue that the simpler architecture and improved instance-feature assignment of DD3Dv2 yield particularly more stable training with shorter schedule. 

\input{tables/dd3d_orig}

\section{Sensitive to loss weights}
We find that, in the case of multi-task training using point-cloud data, detection accuracy is sensitive to the relative weights between the two loss terms (Table~\ref{table:nuscenes-loss-weight}). When the weight for the 3D box loss~\cite{simonelli2019disentangling} is fixed to $1.0$, the optimal value for the depth loss (i.e. mean L1 distance) is $0.45$. The depth accuracy is insensitive to these values.

%In this section, we provide supplemental ablation on the sensitivity of the multi-task performance with respect to the weight of self-supervised $L1$ depth. 
%We report AP and NDS for 3D object detection as well as Abs. Rel for depth estimation on foreground for reference.

% \begin{table}[t!]
% \centering
% {
% \footnotesize
% \setlength{\tabcolsep}{0.4em}
% \rowcolors{2}{lightgray}{white}
% \begin{tabular}{l|c|c|c}
% \toprule
% Class & 
% PointPillars~\cite{lang2019pointpillars} &
% MonoDIS (multi)~\cite{simonelli2020disentangling} &
% FCOS-3D \\
% \midrule

% Barrier      & 39.0   & 50.0 & - \\
% Bicycle      & 1.0    & 25.0 & - \\
% Bus          & 28.0   & 15.0 & - \\
% Car          & 68.0   & 46.0 & - \\
% Constr. Veh. & 4.0    & 6.0  & - \\
% Motorcycle   & 27.0   & 30.0 & - \\
% Pedestrian   & 60.0   & 36.0 & - \\
% Traffic Cone & 31.0   & 49.0 & - \\
% Trailer      & 23.0   & 16.0 & - \\
% Truck        & 23.0   & 21.0 & - \\
% \midrule
% Mean AP [\%] $\uparrow$ & 31.0 & 30.0 & - \\

% % \bottomrule
% \end{tabular}\\\vspace{0mm}
% \caption{
% \textbf{3D detection performance on the nuScenes~\cite{caesar2020nuscenes} test set for all the classes.} We report the \textit{Average Precision} for each class, and the Mean AP over all the classes for each method.}
% \label{table:nuscenes_test_summary}
% }
% \end{table}

\begin{table}[h]
% wandb report;
\centering
{
\tiny
\footnotesize
\setlength{\tabcolsep}{0.3em}
\rowcolors{2}{lightgray}{white}
\begin{tabular}{c|cc|c}
\toprule
Loss Weight& AP[$\%$]$\uparrow$ &  NDS$\uparrow$ & Abs. Rel $\downarrow$ \\
\midrule
0.55 &{38.0} &  {0.45}&\textbf{0.20}\\
%https://wandb.ai/tri/multitask/runs/2evxwhiv
0.45 &\textbf{39.1} &  {\textbf{0.46}}& \textbf{0.20}\\
%https://wandb.ai/tri/multitask/runs/12wsqej2
0.35 &{38.9} &  {0.45}&\textbf{0.20}\\
%https://wandb.ai/tri/multitask/runs/3v47xod0
0.25 &{38.1} &  {0.44}&\textbf{0.20}\\
%https://wandb.ai/tri/multitask/runs/1sll4iek
0.15 &{37.9} &  {0.44}&0.21\\
%https://wandb.ai/tri/multitask/runs/3aiypfed
\midrule
0 &35.8 &0.41 &-\\
%https://wandb.ai/tri/multitask/runs/3aiypfed
 \bottomrule
\end{tabular}\\\vspace{2mm}
\caption{Detection accuracy vs. depth loss weight. We fix the weight for 3D box loss to $1.0$, and search for the optimal value for depth loss in case of our multi-task training using point-cloud.}
\label{table:nuscenes-loss-weight}
}
\end{table}

\section{Detailed results on nuScenes}
In Table~\ref{table:nuscenes_test_detailed}, we present a more detailed version of Table~\ref{table:nuscenes_test_summary}, highlighting the performance on three major categories of  the dataset. Our detectors yield larger improvements in these categories and in stricter evaluation (i.e. $0.5$m threshold). The point-cloud supervision yields larger improvement over the two-stage adaptation.

\begin{table*}[]
\centering
{
\setlength{\tabcolsep}{4.5pt}
\footnotesize
\rowcolors{2}{lightgray}{white}
\begin{tabular}{l|cccc|cccc|cccc}
\toprule
& \multicolumn{4}{c}{Car [\%] $\uparrow$} & \multicolumn{4}{c}{Pedestrian [\%] $\uparrow$} &  \multicolumn{4}{c}{Bicycle [\%] $\uparrow$} \\

\multirow{-2}{*}{Methods}& 
0.5m & 1.0m & 2.0m & 4.0m & 0.5m & 1.0m & 2.0m & 4.0m & 0.5m & 1.0m & 2.0m & 4.0m\vspace{0.5mm}\\

\midrule

% CenterNet$^*$  &
% 20.0 & 45.8 & 68.0 & 80.6 &
% 7.9 & 26.7 & 49.6 & 65.9 &
% 4.3 & 13.8 & 28.4 & 36.2 \\

% AIML-ADL$^*$ &
% 14.2 & 36.8 & 58.5 & 71.0 &
% 9.6 & 30.8 & 54.6 & 69.4 &
% 5.2 & 21.6 & 37.3 & 46.2 \\

% DHNet$^*$ &
% 15.2 & 37.9 & 59.4 & 71.5 &
% 10.5 & 31.7 & 55.7 & 69.9 &
% 5.6 & 24.2 & 38.9 & 48.0 \\

% PGDepth$^*$    &
% 17.0 & 43.6 & 67.2 & 80.3 &
% 9.1 & 31.0 & 53.9 & 69.1 &
% 7.6 & 24.1 & 40.1 & 49.2 \\
MonoDis~\cite{simonelli2019disentangling} &
10.7 &
37.5 &
{69.0} &
{85.7} &
- &
- &
- &
- &
- &
- &
- &
- \\
% MonoDis (multi)~\cite{simonelli2020disentangling} & 
% 10.6 & 36.1 & 65.0 & 80.5 &
% 6.7 & 30.0 & 48.5 & 64.7 &
% 4.4 & 17.5 & 32.8 & 43.9 \\
FCOS3D~\cite{wang2021fcos3d}    &
{15.3} & {43.8} & 68.9 & 81.7 &
{8.7} & {30.3} & {52.9} & {67.1} & 
{7.9} & {25.0} & {39.2} & {47.1} \\
PGD\cite{wang2022probabilistic}    &
{20.4} & {48.7} & 71.8 & 83.4 &
{11.6} & {35.0} & {58.0} & {71.9} & 
{9.7} & {26.2} & {40.4} & {49.1} \\
DD3D~\cite{park2021dd3d} &
{30.2} &
{59.7} &
{77.4} &
{84.1} &
{18.7} &
{42.4} &
{61.9} &
{70.2} &
{15.7}  &
{32.6} &
{45.2} &
{50.0} 
\\
DETR3D~\cite{detr3d}   &
24.1 & 56.2 & {78.1} & {86.7} &
 12.8& 37.3 & 61.6 & {74.3} & 
 10.6& 25.9 & 39.5 & 44.9 \\
\midrule
% unpublished method
BEVDet$^*$~\cite{huang2021bevdet}&
{31.6} & {62.3} & 78.7& 84.3 &
{17.8} & {37.2} & {51.2} & {58.1} & 
{13.5} & {29.0} & {36.6} & {39.1} \\
PETR$^*$~\cite{liu2022petr}     &
{29.6} & {57.8} & 78.1 & \textbf{86.8} &
{13.5} & {39.1} & {62.7} & {74.6} & 
{10.2} & {27.1} & {40.2} & {45.1} \\
\midrule
%"car": {"0.5": 0.3130879826412605, "1.0": 0.600097385413361, "2.0": 0.7806188249781087, "4.0": 0.8520682001205703},
DD3Dv2-Selsup. &{31.3} & {60.0} & {78.1} &85.2
%"pedestrian":{"0.5": 0.19124375823585954, "1.0": 0.43211403004056936, "2.0": 0.627885037024185, "4.0": 0.7299405356391677}, 
 & {19.1} & {44.2} & {62.8} & 73.0 &
%"bicycle": {"0.5": 0.17546062864084366, "1.0": 0.3353361838200302, "2.0": 0.4685883655445414, "4.0": 0.5252648363200102}, 
{17.5} & {33.5} & {46.9} & {52.5} \\
%
%"car": {"0.5": 0.3596536094332398, "1.0": 0.6307015909262296, "2.0": 0.7949206469445562, "4.0": 0.8612389284170383}, 
DD3Dv2 & \textbf{40.0} & \textbf{63.1} & \textbf{79.5} & {86.1}
%"pedestrian": {"0.5": 0.25586117613785087, "1.0": 0.4906324224874566, "2.0": 0.6662985816131062, "4.0": 0.7533312191925321},
 & \textbf{25.6} & \textbf{49.1} & \textbf{66.6} & \textbf{75.3} &
%"bicycle": {"0.5": 0.22941239538697897, "1.0": 0.40273232048042373, "2.0": 0.4965852696170633, "4.0": 0.5323647561498759},
\textbf{22.9} & \textbf{40.3} & \textbf{49.7} & \textbf{53.2}

\end{tabular}\\\vspace{0mm}
\caption{
\textbf{Detailed results on the nuScenes \textit{test} set.} We report mean AP metrics on \emph{Car}, \emph{Pedestrian}, and \emph{Bicycle} with varying thresholds on distance. The \textbf{bold} denotes the best of all.
%\textbf{DD3D detection results on the nuScenes~\cite{caesar2020nuscenes} test set:} we report detailed results on the \textit{Car}, \textit{Pedestrian} and \textit{Bicycle} classes; detailed results for the other classes can be found in the supplementary. * denotes results reported from  the nuScenes official test set that do not have an associated publication at the time of writing.
}
\label{table:nuscenes_test_detailed}
}
\end{table*}

%\section{Model complexity}
%\input{tables/complexity}

\section{Visualization}
We provide a visualization of our detectors in Fig.~\ref{fig:visualization}. We randomly pick examples from the nuScenes \emph{validation} split.

\begin{figure*}[h]
\centering
\subfloat{{\includegraphics[width=\textwidth]{figures/images/fig-3-gt.png} }}\\
\subfloat{{\includegraphics[width=\textwidth]{figures/images/fig-3-sup.png} }}\\
\subfloat{{\includegraphics[width=\textwidth]{figures/images/fig-3-selfsup.png} }}\\
\caption{\textbf{Visualization of detectors.} The \textbf{top} row shows the ground-truth 3D boxes on 4 images in nuScenes \emph{validation} split. The \textbf{middle} and \textbf{bottom} rows shows the detection from our approaches, multi-task training using point-cloud data and our two-stage pseudo-labels approach, respectively. In the top-down view on the upper-right corners, we show the ground-truth (\textbf{green}) overlaid with the detection (\textbf{red}).}
\label{fig:visualization}
\end{figure*}
